# Supplementary material for: A Survey of State of the Art Large Vision Language Models: Alignment, Benchmark, Evaluations and Challenges
Source: arXiv:2501.02189 source file (2026-08-22)
Supplement: Supplementary file 1 [file 60_supplementary.tex]

\clearpage
\setcounter{page}{1}
\maketitlesupplementary

\section{Rationale}
\label{sec:rationale}
Having the supplementary compiled together with the main paper means that:
\begin{itemize}
\item The supplementary can back-reference sections of the main paper, for example, we can refer to \cref{sec:intro};
\item The main paper can forward reference sub-sections within the supplementary explicitly (e.g. referring to a particular experiment); 
\item When submitted to arXiv, the supplementary material will already included at the end of the paper.
\end{itemize}
To split the supplementary pages from the main paper, you can use \href{https://support.apple.com/en-ca/guide/preview/prvw11793/mac#:~:text=Delete%20a%20page%20from%20a,or%20choose%20Edit%20%3E%20Delete).}{Preview (on macOS)}, \href{https://www.adobe.com/acrobat/how-to/delete-pages-from-pdf.html#:~:text=Choose%20%E2%80%9CTools%E2%80%9D%20%3E%20%E2%80%9COrganize,or%20pages%20from%20the%20file.}{Adobe Acrobat} (on all OSs), as well as \href{https://superuser.com/questions/517986/is-it-possible-to-delete-some-pages-of-a-pdf-document}{command line tools}.

\begin{table*}
\centering
\small

\scalebox{0.5}{
\begin{tabular}{p{0.15\textwidth}p{0.18\textwidth}p{0.30\textwidth}p{0.15\textwidth}p{0.08\textwidth}}
\hline
\textbf{Benchmark} & \textbf{Evaluation} & \textbf{Category} & \textbf{Annotation} & \textbf{Size (K)} \\
\hline
MMTBench & Multiple Choice & Visual reasoning & AI Experts & 30.1 \\
MM-Vet & LLM Eval & Visual reasoning & Human & 0.2 \\
MM-En/CN & Multiple Choice & Visual reasoning / Multilingual understanding & Human & 3.2 \\
GQA & Answer Matching & Visual reasoning & Seed with Synthetic & 22,000 \\
VCR & Multiple Choice & Visual reasoning, & MTurks & 290 \\
VQAv2 & Answer Matching\newline Yes/No & Chart graphic understanding & MTurks & 1,100 \\
MMMU & Answer Matching \newline Multiple Choice & Chart graphic understanding & College Students & 11.5 \\
SEEDBench & Multiple Choice & Visual reasoning & Synthetic & 19 \\
RealWorld QA & Multiple Choice & Visual reasoning, understanding, recognition, and question answering & Human & 0.765 \\
MMMU-Pro & Multiple Choice & Visual reasoning & Human & 3.64 \\
DPG-Bench & Semantic Alignment & Visual reasoning / Text2Image generation & Synthetic & 1.06 \\
MSCOCO-30K & BLEU\newline Rouge\newline Similarity & Visual reasoning / Text2Image generation & MTurks & 30 \\
TextVQA & Answer Matching & Visual text understanding & CrowdSource & 45 \\
DocVQA & Answermatching & Visual text understanding & CrowdSource & 50 \\
CMMLU & Multiple Choice & Multilingual multi-modal understanding & College Students & 11.5 \\
C-Eval & Multiple Choice & Multilingual multi-modal understanding & Human & 13.9 \\
TextVQA & Answer Matching & Visual text understanding & Expert Human & 28.6 \\
MathVista & Answer Matching \newline Multiple Choice & Visual math reasoning & Human & 6.15 \\
MathVision & Answer Matching \newline Multiple Choice & Visual math reasoning & College Students & 3.04 \\
OCRBench & Answer Matching & OCR & Human & 1 \\
MME & Yes/No & OCR & Human & 2.8 \\
InfographicVQA & Answer Matching & Chart graphic understanding & CrowdSource & 30 \\
AI2D & Answer Matching & Chart graphic understanding & CrowdSource & 1 \\
ChartQA & Answer Matching & Chart graphic understanding & CrowdSource;synthetic & 32.7 \\
GenEval & CLIPScore \newline GenEval & Text-to-Image generation & MTurks & 1.2 \\
T2I-CompBench & Multiple Metrics & Text-to-Image generation & Synthetic & 6 \\
HallusionBench & Yes/No & Hallucination & Human & 1.13 \\
POPE & Yes/No & Hallucination & Human & 9 \\
MMLU & Multiple Choice & Multimodal general intelligence & Human & 15.9 \\
MMStar & Multiple Choice & Multimodal general intelligence & Human & 1.5 \\
M3GIA & Multiple Choice & Multimodal general intelligence & Human & 1.8 \\
InternetAGIEval & Multiple Choice &Multimodal general intelligence & Human & 8.06 \\
EgoSchem & Multiple Choice & Video understanding & Synthetic/Human & 5 \\
MVBench & Multiple Choice & Video understanding & Synthetic/Human & 4 \\
MLVU & Multiple Choice & Video understanding & Synthetic/Human & 2.6 \\
VideoMME & Multiple Choice & Video understanding & Experts & 2.7 \\
Perception-Test & Multiple Choice & Video understanding & CrowdSource & 11.6 \\
VQAScore & Yes/No & Vision-Language Alignment & AI & 665 \\
GenAI-Bench & Human Ratings  & Generative AI Evaluation & Human & 80.0 \\
NaturalBench & Yes/No \newline Multiple Choice & Vision-Language Adversarial Testing & Human & 10.0 \\
\hline
\end{tabular}
}
\caption{Benchmarks and evaluations, along with their annotation and data source.}
% \caption{Benchmarks and evaluations, along with how they are annotated and where their data come from.}
\label{tab:benchmark-eval}
\vspace{-0.5 cm}
\end{table*}
